# Supplementary material for: Measuring Cosmic Neutrino Masses Independently of Dark Energy
Source: arXiv:2607.24742 source file (2026-07-27)
Supplement: Supplementary file 1 [file supplementary.tex]

	% \onecolumngrid
	\begin{center}
		\textbf{\large{\textit{Supplementary Material}}}\\
		\hfill \break
		\smallskip
	\end{center}

\section{Analytic estimate of the covariance matrix}\label{app.covmat}
We estimate the joint covariance between SPT-3G and \textit{Planck} CMB lensing.  Correlations arise not only from the shared underlying gravitational potential being measured, but also from the reconstruction noise $n_0$ since part of this is sourced by the same CMB fluctuations that mimic lensing. Given that the full SPT-3G footprint is enclosed within the \textit{Planck} footprint, we decompose the \textit{Planck} convergence field as follows: 

\begin{equation}
    \kappa^{P}(\hat{n}) 
= 
\begin{cases}
 \kappa_{\mathrm{in}}(\hat{n}) + n^P_{{\mathrm{in},0}}(\hat{n}), 
       & \text{inside SPT patch},\\[6pt]
   \kappa_{\mathrm{out}}(\hat{n}) + n^P_{{\mathrm{out},0}}(\hat{n}), 
       & \text{outside SPT patch}.
\end{cases}
\end{equation}

Here $\kappa_{\mathrm{in}}(\hat{n})$ is the lensing field on the SPT overlap region, $\kappa_{\mathrm{out}}(\hat{n})$ is on the rest of \textit{Planck} sky and $n^p$ denotes the \textit{Planck} reconstruction noise.

For SPT-3G we have 

\begin{equation}
    \kappa^{S}(\hat{n}) 
= 
\begin{cases}
   \kappa_{\mathrm{in}}(\hat{n}) + n^S_{{\mathrm{in},0}}(\hat{n}), 
       & \text{inside SPT patch},\\[6pt]
   0  
       & \text{outside SPT patch}.
\end{cases}
\end{equation}

From the definitions above, it is clear that only the overlapping region between both surveys contributes to their correlation and thus the covariance matrix. For simplicity, we drop the subscript "in" going forward, noting explicitly that $\kappa(\hat{n})$ and $n_0$ refers exclusively to the overlap region between SPT-3G and \textit{Planck}.

For the analytic covariance between the two measured lensing spectra $\hat{C}^{\kappa_P\kappa_P}_L$ and $\hat{C}^{\kappa_S\kappa_S}_L$, we have from Wick's theorem

\begin{equation}
    \mathrm{Cov}(\hat{C}^{\kappa_P\kappa_P}_L,\hat{C}^{\kappa_S\kappa_S}_L)=\frac{2}{(2L+1)f_\mathrm{\mathrm{sky,overlap}}}(\hat{C}^{\kappa_P\kappa_S}_L)^2.
\end{equation}

The correlation coefficient within the overlap for the two surveys is then given by

\begin{equation}
    \rho^{\mathrm{overlap}}_L(P,S)=\frac{\mathrm{Cov}(\hat{C}^{\kappa_P\kappa_P}_L,\hat{C}^{\kappa_S\kappa_S}_L)}{\sqrt{\mathrm{Var(\hat{C}^{\kappa_P\kappa_P}_L)}}\sqrt{\mathrm{Var(\hat{C}^{\kappa_S\kappa_S}_L)}}}
\end{equation}

The denominator can be obtained from the raw non-bias subtracted reconstructions of the different instruments in the overlap region. To calculate the full correlation coefficient accounting for the decorrelation due to the difference in area, one simply needs to rescale $\rho^{\mathrm{overlap}}_L(P,S)$ accounting for the different $f_\mathrm{sky}$ of the different footprints.

\begin{equation}
    \rho^{}_L(P,S)=\frac{f^\mathrm{overlap}_\mathrm{sky}}{\sqrt{f^\mathrm{S}_\mathrm{sky}f^\mathrm{P}_\mathrm{sky}}}\rho^{\mathrm{overlap}}_L(P,S)
\end{equation}

For the numerator $\hat{C}^{\kappa_S\kappa_P}_L$,
if we have assumed that the reconstruction noise is uncorrelated between SPT and \textit{Planck}, 
$N_L^{\kappa_P\kappa_S} \;\equiv\; \bigl\langle n^P\,n^S \bigr\rangle_L = 0$, then it is just $(C^{\kappa\kappa}_L)^2$ without any reconstruction noise, corresponding to the lower bound in the estimate of the correlation coefficient shown in  \textcolor{blue}{dashed blue} in the left panel of Fig.~\ref{fig. corr_coeff}.

However, we do expect the signal component of the \textit{Planck} polarization only (MVPOL) reconstruction noise to be correlated with the signal part of the SPT-3G reconstruction noise (which is polarization only) due to common CMB modes. If one naively assumes that all the signal part of the \textit{Planck} reconstruction noise bias ($N_0$) correlates with the SPT-3G $N_0$, then $\hat{C}^{\kappa_P\kappa_S}_L={C}^{\kappa\kappa}_L+N^{SPT}_L$, i.e., the reconstruction noise power spectrum from the SPT-3G measurement. For illustration, this is shown as the \textcolor{red}{dashed red} curve in the left panel of Fig.~\ref{fig. corr_coeff}, which will be an overestimate since the polarization contribution to the \textit{Planck} $\hat{\kappa}$ is subdominant to the temperature channel. A quick estimate of the fraction of the MVPOL lensing reconstruction in \textit{Planck} is given by 
\begin{equation}
    f_\mathrm{MVPOL}=\frac{\sum_{XY\in\{EE,EB\}}\mathcal{R}^{XY}_L}{\sum_{XY}{\mathcal{R}^{XY}_L}}
\end{equation}
i.e. the ratio of the inverse MVPOL normalization to the inverse of the minimum-variance (MV) normalization, where $XY \in [TT, TE, EE, EB, TB]$. Thus the cross-reconstruction noise power spectrum is given by $\langle{n^\mathrm{signal,S}_0+n^\mathrm{noise,S}_0,    f_\mathrm{MVPOL}(n^\mathrm{signal,P}_0}+n^\mathrm{noise,P}_0)\rangle=f_\mathrm{MVPOL}N^\mathrm{signal,SPT}_0\leq{f_\mathrm{MVPOL}N^\mathrm{SPT}_0}$. We approximate the numerator term as $\hat{C}^{\kappa_P\kappa_S}_L={C}^\mathrm{\kappa\kappa}_L+f_\mathrm{MVPOL}{N}^\mathrm{SPT}_L$ noting that this will be an upper bound since the instrument noise part of the SPT $N_0$ will not appear in reality. This upper bound is shown in \textbf{black} in the left panel of Fig. \ref{fig. corr_coeff}.

We repeat the same calculation to estimate the correlation between ACT and SPT-3G. Noting that in this case, for the correlation due to reconstruction noise $\langle{n^\mathrm{signal,S}_0+n^\mathrm{noise,S}_0,    f^\mathrm{A}_\mathrm{MVPOL}(n^\mathrm{signal,A}_0})\rangle=f^\mathrm{A}_\mathrm{MVPOL}N^{ \mathrm{signal,ACT}}_0$, one can use the realization dependent $N_0$ of ACT that does not have contribution from instrument noise to estimate a more accurate correlation due to the signal contribution to the reconstructed noise.

\begin{figure}[h!]
    \centering    \includegraphics[width=\columnwidth]{figures/correlation.pdf}
    \caption{\textbf{Left}: Correlation coefficient estimates between \textit{Planck} and SPT-3G. In solid black, we show the analytic correlation coefficient used to generate the off-diagonal covariance matrix between \textit{Planck} and SPT. We also show in the dashed blue line an underestimate of this correlation coefficient when the correlated part of the reconstruction noise between the two experiments is not included. In red we show an unrealistic pessimistic estimate of the correlation coefficient where we assume the reconstruction noise of both surveys is fully correlated.
    \textbf{Right}:  Analogous estimates for ACT DR6 and SPT-3G.  Note that in this case, the analytic correlation coefficient used (black) enables us to use the ACT MVPOL RDN0 (that only has the signal contribution to the reconstruction noise) as an estimate of the true correlation between the two surveys' reconstruction noise; as expected, this is lower than the orange curve (calculated similarly to the black curve in the left plot) in the signal-dominated regime. }
    \label{fig. corr_coeff}
\end{figure}

We convert the analytical estimates of the correlation coefficients into the off-diagonal elements of the covariance matrix. Although these analytic estimates do not explicitly account for correlations between non-overlapping bins, we only expect significant correlations for bins where the bandpowers of the different surveys overlap in multipole space. For overlapping bins, we assign a correlation coefficient, $\rho$, at the multipole corresponding to the average of the two survey bin centres. For bin pairs whose centers differ by more than 50, we set $\rho=0$, since we do not expect any significant correlation between non-overlapping bins. (The use of realization dependent $N_0$ ensures that off-diagonal correlations are kept at a minimum \citep{PhysRevD.83.043005,Schmittfull_2013}.) In Figure~\ref{fig.comparison}, we compare parameter constraints under three scenarios: excluding off-diagonal contributions between SPT and both \textit{Planck} and ACT (green), using the baseline analytic correlations (blue) and employing the unrealistic pessimistic correlations described above (orange). Notably, even in the pessimistic unrealistic scenario, including the off-diagonal components has only a minimal effect compared to omitting them entirely.

\begin{figure}[h!]
    \centering    \includegraphics[width=\columnwidth]{figures/corr_act_spt.pdf}
    \caption{Binned correlation coefficient for ACT-SPT-3G and \textit{Planck}-SPT-3G used in the covariance matrix of the likelihood.}
    \label{fig. corr_coeff_matrix}
\end{figure}

\begin{figure}[h!]
    \centering    \includegraphics[width=0.8\columnwidth]{figures/comparison.pdf}
    \caption{Comparison of parameter constraints obtained under three different treatments of off-diagonal covariance components between SPT-3G M2PM and both \textit{Planck} PR4 and ACT DR6. The green curves show constraints when off-diagonal contributions are omitted entirely, the blue curves correspond to the baseline analytic correlation model and the orange curves depict a pessimistic scenario assuming full correlation for overlapping bins. Even in the pessimistic case, the impact of including off-diagonal terms is minimal compared to neglecting them.}
    \label{fig.comparison}
\end{figure}

\section{Results using alternative BAO datasets}\label{app.variation}
We explore three variants of BAO datasets in this analysis. They are Pre-DESI BAO, DESI DR1 BAO  and Hybrid BAO, defined as follows. 
Pre-DESI BAO and Hybrid BAO are included for comparisons with the results produced in the ACT DR6 lensing~\cite{ACT:2023dou,ACT:2023kun,ACT:2023ubw} and the \sptshort~\citep{SPT-3G:2024atg} papers, respectively. The parameter constraints from CMB lensing with these BAO datasets are samarized in Table~\ref{tab:params2}.
\begin{itemize}
    \item Pre-DESI BAO consists of BAO  measurements from 6dFGS \cite{2011MNRAS.416.3017B}, SDSS DR7 MGS \cite{1409.3242}, BOSS DR12 LRGs \cite{1607.03155} and eBOSS DR16 LRGs \cite{2007.08991}. 
    \item DESI DR1 BAO denotes the DESI-Y1 release \cite{desicollaboration2024desi}, covering redshifts $0.1\leq{z}\leq4.2$ with samples including BGS, LRG, ELG, QSO and the Lyman-$\alpha$ forest.
    \item Hybrid BAO is based on the DESI BAO set but replaces the DESI BGS and lowest redshift DESI LRG with SDSS MGS $(z_\mathrm{eff}\sim0.15)$ and two BOSS DR12 LRG points at $(z_\mathrm{eff}\sim0.38,0.51)$. The DESI Ly$\alpha$ point is also replaced with the joint eBOSS+DESI DR1 Ly$\alpha$ BAO. The 6dFGS BAO measurement is also included here. 
\end{itemize}

In combination with APS lensing, they result in the following $\sigma_8$ constraints
\begin{eqnarray}
    \sigma_8 &=& 0.827 \pm 0.010\\ \nonumber &&({\rm ACT}+\textit{Planck}+{\rm SPT}+ {\rm hybrid\, BAO}),\\
    \sigma_8 &=& 0.821 \pm 0.010\\ \nonumber &&({\rm ACT}+\textit{Planck}+{\rm SPT}+ {\rm pre\text{-}DESI\, BAO})\text{\ and}\\
    \sigma_8 &=& 0.831 \pm 0.010\\ \nonumber &&({\rm ACT}+\textit{Planck}+{\rm SPT}+ {\rm DESI \,DR1\, BAO}).
\end{eqnarray}

From the combination of the joint CMB lensing,  galaxy BAO and the $\Omega_bh^2$ prior in Table~\ref{table:priors}, we obtain a $1.1$--$1.4\%$ constraint on $H_0$:
\begin{eqnarray}
    H_0 &=& 68.46\pm 0.73 \hun\\ \nonumber &&({\rm ACT}+\textit{Planck}+{\rm SPT}+ {\rm hybrid\, BAO}),\\
    H_0 &=& 68.42\pm 0.98 \hun\\ \nonumber &&({\rm ACT}+\textit{Planck}+{\rm SPT}+ {\rm pre\text{-}DESI\, BAO})\text{\ and}\\
    H_0 &=& 69.15\pm 0.74 \hun\\ \nonumber &&({\rm ACT}+\textit{Planck}+{\rm SPT}+ {\rm DESI \,DR1 \, BAO}).
\end{eqnarray}

\begin{table}[ht]
%\begin{ruledtabular}
\begin{tabular}{l  c  c  c } \hline\hline
Experiment & $S^{\mathrm{lens}}_8$ & $\sigma_8$ & $\Omega_m$ \\
\hline
A+ pdBAO & $0.829 \pm 0.020$ & $0.819 \pm 0.015$ & $0.315 \pm 0.016$ \\
S+ pdBAO  & $0.836 \pm 0.012$ & $0.821 \pm 0.013$ & $0.323 \pm 0.018$ \\
{P} + pdBAO & $0.822\pm0.021$  & $0.814\pm0.016$ &  $0.313^{+0.014}_{-0.017}$\\
AS+pdBAO & $0.836 \pm 0.011$ & $0.823 \pm 0.011$ & $0.319 \pm 0.014$ \\
APS+ pdBAO & $0.828 \pm 0.010$ & $0.831 \pm 0.010$ & $0.317 \pm 0.012$ \\
APS+ DESI DR1 BAO & $0.832 \pm 0.010$ & $0.821 \pm 0.010$ & $0.296 \pm 0.010$ \\
APS+ hBAO & $0.828^{+0.011}_{-0.010}$ & $0.827 \pm 0.010$ & $0.302^{+0.009}_{-0.010}$ \\
APS+ DESI DR2 BAO & $0.829^{+0.009}_{-0.009}$ & $0.829 \pm 0.009$ & $0.300\pm0.007$\\
\hline
\end{tabular}
%\end{ruledtabular}
\caption{Cosmological parameter measurements from the various lensing experiment combinations. We use A, {P} and S as shorthands for CMB lensing with ACT DR6, \textit{Planck} PR4 and \sptshort\ respectively. pdBAO refers to pre-DESI BAO and hBAO stands for hybrid BAO.}
\label{tab:params2}
\end{table}

\section{$\sigma_8$ Constraints from galaxy and CMB lensing}\label{sec:sig8}
In Fig.~\ref{fig:sigma8}, we compare the $\sigma_8$ constraints from galaxy and CMB lensing in combination with BAO measurements. Since CMB lensing measurements extend a large range of angular scales, while the galaxy lensing is mostly sensitive to the structure growth at small scales, CMB lensing is more constraining than galaxy lensing on $\sigma_8$ \cite{ACT:2023kun}.

\begin{figure}
    \centering
    \includegraphics[width=0.8\linewidth]{figures/sigma8_constraints.pdf}
    \caption{
    Constraints on $\sigma_8$ inferred from galaxy lensing surveys of DES-Y3 \cite{DES:2021bvc, DES:2021vln, DES:2021wwk}, KiDS-1000 \citep{KiDS:2020suj, Heymans:2020gsg} and HSC-Y3 \citep{Li:2023tui, Dalal:2023olq} (plus BAO), as well as KiDs-Legacy \citep{Wright:2025xka, Stolzner:2025htz} (plus BAO and supernovae),  CMB lensing (plus BAO) and CMB primary spectra from \textit{Planck} PR3 and \textsf{P-ACT}. 
    %\KW{Need a line to describe the KiDS-Legacy set. It's different from the HSC/DES/KiDS1000 above because this also has SNe.}
    The blue errorbars show the constraints under the $\Lambda\mathrm{CDM}$ model, while the red errorbars are inferred for a $\Lambda\mathrm{CDM}+\sum m_\nu$ model. The constraints derived from \textit{Planck} 2018 \texttt{TTTEEE lowl lowE} are labeled as Planck T\&E. The vertical gray band also shows the 1 and 2$\sigma$ regions inferred from Planck T\&E assuming $\Lambda\mathrm{CDM}$.
    %The recent KiDS-Legacy result \citep{Wright:2025xka, Stolzner:2025htz} shows agreement in the $S_8$ constraint with the  \textit{Planck} primary CMB. While not included in the figure, we expect the KiDS-Legacy lensing + BAO $\sigma_8$ constraint to shift toward the \textit{Planck}-inferred value.
    }
    \label{fig:sigma8}
\end{figure}
